# Supplementary material for: Structural-RNN: Deep Learning on Spatio-Temporal Graphs
Source: arXiv:1511.05298 source file (2016-04-11)
Supplement: Supplementary file 1 [file supplementary_tech.tex]

\subsection{Old writeup}
Our goal is to represent the spatio-temporal graph described above with a deep learning architecture.  We approach this problem by parameterizing the node and edge factors of the spatio-temporal graph with Recurrent Neural Networks (RNNs).  We refer the RNNs obtained in this manner as nodeRNNs and edgeRNNs respectively. Our final structural-RNN architecture captures the structure of the spatio-temporal graph through connections between the edgeRNNs and nodeRNNs. Each edgeRNN in our architecture handles a specific kind of interaction between nodes, and each nodeRNN combines the outputs of edgeRNNs it is connected to and predicts the node labels. The key insight in connecting edgeRNNs to nodeRNNs is to appropriately combine and edge and node observations for every node before predicting the labels.

In order to capture the structure of the spatio-temporal graph we connect the edgeRNNs and nodeRNNs to form a bipartite graph which we call the structural-RNN architecture.  Each edgeRNN in our architecture handles a specific kind of interaction between nodes, and each nodeRNN combines the outputs of edgeRNNs it is connected to and predicts the node labels. The key insight in connecting edgeRNNs to nodeRNNs is to appropriately combine and edge and node observations for every node before predicting the labels.

Our architecture begins with parameterizing shared node factors $\Psi_{V_p}$ and edge factors $\Psi_{E_m}$, $\Psi_{{\bar{E}_n}}$ with RNNs. We denote the RNN parameterization of $\Psi_{V_p}$ with $\ve{R}_{V_p}$ and refer to it as \textit{nodeRNN}. Likewise $\ve{R}_{E_m}$ and $\ve{R}_{\bar{E}_n}$ denote the \textit{edgeRNNs} associated with the edge factors $\Psi_{E_m}$ and $\Psi_{\bar{E}_n}$ respectively. Intuitively, edgeRNNs serves the purpose of representing the spatial and temporal interactions between the nodes of the spatio-temporal graph. Each edgeRNN is dedicated to handle a specific kind of node interaction. On the other hand, each nodeRNN is connected to multiple edgeRNNs and it temporally fuses their outputs to predict the node labels. The key to capturing the structure of the spatio-temporal graph lies in defining connections between the nodeRNNs and edgeRNNs in order to form a structural RNN architecture. 

We connect nodeRNNs and edgeRNNs to form a bipartite graph $\mcal{G}_{\ve{R}} = (\{\ve{R}_{E_m}\}\cup\{\ve{R}_{\bar{E}_n}\},\{\ve{R}_{{V}_p}\},\mcal{E}_R)$ such that the output of edgeRNNs is connected to the input of nodeRNNs. The key insight in establishing connections $\mcal{E}_R$ between nodeRNNs and edgeRNNs is to ensure that when  predicting the label of node $v$ (s.t. $\Psi_v \in {V_p}$) the nodeRNN $\ve{R}_{{V}_p}$ combines the outputs from all the edgeRNNs that represent edge factors $\Psi_{(u,v)}$ with node $v$.
 With this insight we connect edgeRNNs and nodeRNNs in $\mcal{G}_{\ve{R}}$ to capture the structure of the spatio-temporal graph $\mcal{G}$ as follows:
\begin{align}
\nonumber (\ve{R}_{E_m},\ve{R}_{{V}_p}) \in \mcal{E}_R \Longleftrightarrow& \exists u \in \mcal{V} \; \text{\&}\; \exists \Psi_v \in V_p\\
&\text{s.t.}\; \Psi_{(u,v)} \in E_m
\end{align}
The above equation convey that the nodeRNN $\ve{R}_{V_p}$ process the output from the edgeRNN $\ve{R}_{E_m}$ if there is a node $v$ and spatial edge $(u,v) \in \mcal{E}_S$ in the graph such that the node factor $\Psi_v \in {V_p}$ and the edge factor $\Psi_{(u,v)} \in {E_m}$. Likewise the edgeRNNs $\ve{R}_{\bar{E}_n}$ for temporal edges $\mcal{E}_T$ are connected to the nodeRNNs as follows: 
\begin{align}
\nonumber (\ve{R}_{\bar{E}_n},\ve{R}_{{V}_p}) \in \mcal{E}_R \Longleftrightarrow& \exists u' \in \mcal{V} \; \text{\&}\; \exists \Psi_v \in V_p\; \text{s.t.}\\
&\Psi_{(u',v)} \;\text{or}\;\Psi_{(v,u')}\in \bar{E}_n
\end{align}
Our structural RNN architecture is non-markovian and it allows nodeRNNs to non-linearly combine the outputs from multiple edgeRNN in order to predict the nodes' labels. This is in contrast to the parametrization of the spatio-temporal graph discussed in Section~\ref{sec:stgraph} where the node and edge factors only interact through product (or through summations in log-space). In the next section we will formally define the inputs and outputs into the edgeRNNs and nodeRNNs, and how we train the architecture end-to-end. 

\section{Training structured rnn}

So far we have discussed how we represent a spatio-temporal graph with an structural RNN architecture. In order to train the architecture we now define the inputs and outputs of edgeRNNs and nodeRNNs. During training the node labels $y_v^t$ and observations $\ve{x}_v^t$, $\ve{x}_e^t$, and $\ve{x}_{\bar{e}}^t$ are given for the time instants $t=1$ to $T$. For each node $v \in \mcal{V}$ we define sets $\mcal{S}_{v,E_m}$ and $\mcal{S}_{v,\bar{E}_n}$ of spatial edges $(u,v) \in \mcal{E}_S$ and temporal edges $(u',v) \in \mcal{{E}}_T$ such that the edge factors $\Psi_{(u,v)} \in  E_m$ and $\Psi_{(u',v)} \in  \bar{E}_n$ respectively.

\begin{align}
\mcal{S}_{v,E_m} = \{(u,v) | (u,v) \in \mcal{E}_S \; \text{\&}\; \Psi_{(u,v)} \in E_m\} \\
\mcal{S}_{v,\bar{E}_n} = \{(u',v) | (u',v) \in \mcal{E}_T \; \text{\&}\; \Psi_{(u',v)} \in \bar{E}_n\}
\end{align}
In order to predict the label of node $v$ the input into edgeRNN $\ve{R}_{E_m}$ at time $t$ is $\sum_{e \in \mcal{S}_{v,E_m}} \phi_{E_m}(\ve{x}_e^t)$, where $\phi_{E_m}$ is the feature function of the edge factor $\Psi_{E_m}$. If the set $\mcal{S}_{v,E_m}$ is empty then the input into edgeRNN $\ve{R}_{E_m}$ is a vector of $\ve{0}$'s. Similarly the input into edgeRNN  $\ve{R}_{\bar{E}_n}$ at time $t$ is $\sum_{e \in \mcal{S}_{v,\bar{E}_n}} \phi_{\bar{E}_n}(\ve{x}_{\bar{e}}^t)$, where $\phi_{\bar{E}_n}$ is the feature function of the edge factor $\Psi_{\bar{E}_n}$. The output of edgeRNNs $\ve{R}_{E_m}$ and $\ve{R}_{\bar{E}_n}$ at each time step $t$ are high-level representations which we denote as $\ve{h}_{E_m}^t$ and $\ve{h}_{\bar{E}_n}^t$ respectively. In this way edgeRNNs model the interactions of node $v$ with its adjacent nodes. Furthermore each edgeRNN is dedicated to model a specific kind of interaction between nodes. By parameterizing edge factors with Recurrent Neural Networks and Long Short-Term Memory (LSTM) units we allow our architecture  to model the time evolving nature of interactions between the node $v$ and its neighbouring nodes. 

The label of node $v$ where $\Psi_v \in V_p$ is predicted by the nodeRNN $\Psi_{V_p}$ which combines the high-level representations from edgeRNNs it is connected to in the bipartite graph $\mcal{G}_{\ve{R}}$. At time step $t$ the input into the nodeRNN $\Psi_{V_p}$ is  concatenation of: (i) the high-level representations $\ve{h}_{E_m}^t$ and $\ve{h}_{\bar{E}_n}^t$ from edgeRNNs such that $(\ve{R}_{E_m},\ve{R}_{{V}_p}) \in \mcal{E}_R$ and $(\ve{R}_{\bar{E}_n},\ve{R}_{{V}_p}) \in \mcal{E}_R$; with (ii) the feature representation $\phi_{V_p}(\ve{x}_v^t)$ of node observation, where  $\phi_{V_p}$ is the feature function of node factor $\Psi_{V_p}$.
